# Supplementary material for: Analyzing Control Flow Integrity with LLVM-CFI
Source: arXiv:1910.01485 source file (2019-10-02)
Supplement: Supplementary file 1 [file appendix.tex]

% % \paul{How to avoid that a reviewer will say, I need to read the appendix to understand the paper? This is an easy critique point. Are we safe with the current Appendix? What parts to remove from the appendix?}
% % \gang{Good point, but unless you shorten the appendix, I don't see how this can be addressed. IMO, sec 12 in the appendix is not very interesting. Also, it's weird to have "Lessons learned" and "Extended related work" in the appendix; either move it to the main text or remove it. Also change appendix sectioning to A, B, C; right now, it looks like the continuation of the main text. Basically, appendix should only provide complementary info and the main text should tell readers what info is in the appendix and the main text should have forward references to the info in appendix.
% % }

% % In the following, we will present the mapping of callers to callees and a simple ranking of CFI policies w.r.t. their level 
% % of calltarget set restrictiveness.

% % \begin{figure}[H]
% % \centering
% % \captionsetup{singlelinecheck = false, justification=justified}
% %    \includegraphics[width=.95\columnwidth]{odt/overview.pdf}
% %     \caption{Caller/callee mappings \& ranked CFI policies.}
% %     \label{overview}
% %  \end{figure}

% % \autoref{overview} depicts different types of callsites and the allowed calltargets (left) and several CFI policies ranked based on their level of calltarget set restrictiveness. We pursue two goals with this figure. First, we want to highlight which 
% % callsite types can target which callee types under \verb!C++!. Second, we rank CFI policies (right) based on the criteria that less restrictive CFI policies w.r.t. to return target set reduction use fewer program 
% % primitives (\textit{e.g.,} parameter type, pointer types, function name, etc.) for constructing constraints, while stricter policies use more of these program primitives.

% \section{Mapping Defenses Into \sysname} 
% \label{Mapping Defenses Into CFI-Assessor} 
% \input{parts/mapping}

% \section{Assessing CFI Policies}
% % \subsection{Assessing CFI Policies}
% \label{rq6}
% In this section, we present how \sysname 
% performs different types of CFI-related measurements.
% \sysname helps to provide precise and reproducible measurement 
% results when performing CFI-related investigations. This section provides several alternatives to existing limited
% CFI metrics: AIR~\cite{mingwei:sekar}, fAIR~\cite{vtv:tice}, and AIA~\cite{aia}, which provide average result values w.r.t. only forward 
% edges calltarget set reduction per callsite after a certain CFI policy was applied 
% to a program. Further, we will show with which novel CFI-related policies 
% \sysname can be used in conjunction. Another set of metrics was
% introduced in a recent survey by Burow \textit{et al.}~\cite{cfi:survey};
% we evaluate our metrics on real-world programs while in the survey the authors
% evaluate their metrics on a per-mechanism basis, changing the point of view.
% Finally, for space reasons we focus on the most widely used ones.
% % \vspace{-.2cm}
% \begin{figure}[ht]
% \captionsetup{justification=justified}
% \centering
% \tikz \node [scale=.78, inner sep=0] {
%  \begin{tikzpicture}
%   \matrix (m) [matrix of math nodes,row sep=3em,column sep=4em,minimum width=2em]
%   {
% %       \textbf{CSD}  &                & \textbf{bCGA}     &\textbf{RSD}         \\
%                     &                & \textbf{bCGA}     &                    \\
%       \textbf{CTR}  & ics            & irs               &\textbf{RTR}        \\
%       VT            & CH             & CFG               &P                   \\
%       VTH           & \textbf{fCGA}  & CG                &                    \\};
%   \path[-stealth]
%     (m-2-2) edge node [above] {$inside$} (m-3-2) %ICS - CH
%     (m-2-1) edge [dashed] node [above] {$uses$} (m-2-2) %iCTR - ICS
%     (m-2-1) edge [dashed] node [left] {$uses$} (m-3-2) %iCTR - CH
%     (m-3-3) edge node [below] {$abstraction$} (m-3-4) %CFG - P
%     (m-3-1) edge node [above] {$subpart$} (m-4-1) %VT- VTH
%     (m-4-1) edge node [below] {$subpart$} (m-3-2) %VTH - CH
%     (m-3-1.east|-m-3-2) edge node [below] {$subpart$} (m-3-2) %VT- CH
%     (m-3-2.east|-m-3-3) edge node [below] {$abstraction$} (m-3-3) %CH- CFG
%     (m-4-3) edge node [below] {$contained$} (m-3-3) %CG - CFG
% %     (m-1-1) edge [dashed] node [above] {$uses$} (m-2-1) %CSD - iCTR
    
%     (m-4-2) edge [dashed] node [above] {$uses$} (m-3-2) %fCGA - CH
%     (m-4-3) edge [dashed] node [above] {$uses$} (m-4-2) %CG - fCGA
    
% %     (m-1-4) edge [dashed] node [above] {$uses$} (m-2-4) %RSD - iRTR
%     (m-2-4) edge [dashed] node [above] {$uses$} (m-2-3) %iRTR - IR
%     (m-2-3) edge [dashed] node [below] {$uses$} (m-3-2) %IRS - CH
    
%     (m-2-3) edge [dashed] node [above] {$coupled$} (m-2-2) %IRS - ICS
%     (m-1-3) edge [dashed] node [above] {$depends$} (m-2-2) %bCGA - ICS
%     (m-1-3) edge [dashed] node [above] {$uses$} (m-2-3) %bCGA - IRS
    
%     (m-2-4) edge [dashed] node [below] {$uses$} (m-3-2) %iRTR - CH
%     ;
% \end{tikzpicture}};
% % \centering
% \caption{Relationships between our four metrics (bold text), and
% program metadata primitives.}
% \label{Interaction of forward-edge related concepts.}
% \end{figure}

% \autoref{Interaction of forward-edge related concepts.} depicts the relationships between our 
% metrics and program primitives. 
% In \autoref{Interaction of forward-edge related concepts.},
% we use the following abbreviations:
% % \begin{enumerate}[labelindent=0pt]
% %  \item 
% (1) \emph{ics:} indirect call site (\textit{i.e.,} x86 \texttt{call} instruction);
% %  \item 
% (2) \emph{irs:} indirect return site (\textit{i.e.,} x86 \texttt{ret} instruction);
% %  \item 
% (3) \emph{P:} program;
% %  \itedm 
% (4) \emph{VT:} virtual table;
% %  \item 
% (5) \emph{VTI:} virtual table inheritance;
% %  \item 
% (6) \emph{CH:} class hierarchy;
% %  \item 
% (7) \emph{CFG:} control flow graph;
% %  \item 
% (8) \emph{CG:} code reuse gadget;
% %  \item 
% Metrics: (9) \emph{CTR:} indirect call target reduction;
% %  \item 
% % (10) \emph{CSD:} indirect call site damping metric;
% %  \item 
% (10) \emph{RTR:} indirect return target reduction;
% %  \item 
% % (12) \emph{RSD:} indirect return site damping metric;
% %  \item 
% (11) \emph{fCGA:} forward-edge based $CG$ availability;
% %  \item 
% (12) \emph{bCGA:} backward return-edge based $CG$ availability.
% % \end{enumerate}

% Based on the two observations: (1) \sysname allows to determine precise forward edge mappings as
% well as backward edge mappings when the forward edge mapping is available due to the caller callee function
% calling convention, and (2) \sysname can be used to search for the presence of code reuse gadgets 
% (\textit{i.e.,} COOP gadgets which are complete virtual functions).

% Next, we formulate four advantages of our approach:
% (1) our metrics do not provide average numbers but rather absolute values,
% (2) can be used to assess backward edge target set reduction,
% (3) can be used to assess the forward and backward edge control flow transfer damping due to a variable number of checks inserted before each indirect control flow transfer, and
% (4) can be used to assess the forward and backward edge control flow transfers w.r.t. gadget availability. 
% Finally, we present our four CFI metrics which can be used in conjunction with \sysname.

% \newcommand{\ctr}{\mathit{ctr}}

% \begin{definition}[\textbf{CTR}]
% Let $ics_{i}$ be a particular indirect callsite in a program $P$,
% $\ctr_{i}$ is the total number of legitimate calltargets for an $ics_{i}$ 
% after hardening a program with a certain CFI policy.
% \label{ctr label}
% \end{definition}
% Then the $iCTR$ metric is:
% % \begin{equation}
% $CTR = \sum_{i=1}^n \ctr_{i}$.
% % \end{equation}
% Note that the lower the value of $CTR$ is for a given program, the more precise the CFI policy 
% is. The optimal value of this metric is equal to the total number of callsites present 
% in the hardened program. This means that there is a one-to-one mapping.
% We can also capture the distribution of the numbers of call targets
% using min, max, and standard deviation functions.

% Minimum: $\min_{i}{\{\ctr_{i}\}}$;
% Maximum: $\max_{i}{\{\ctr_{i}\}}$; and
% Standard Deviation (SD): $CTR_{SD} = \sqrt{\frac{\sum_{i=1}^n ({ctr_{i} - \overline{ctr_{i}}})^2}{n}}\label{ctrsd}$.

% \begin{definition}[\textbf{RTR}]
% Let $irs_{i}$ be a particular indirect return site in the program $P$,
% $rtr_{i}$ is the total number of available return targets for each $irs_{i}$ 
% after hardening the backward edge of a program with a CFI policy.
% \label{rtr definition.}
% \end{definition}
% Then the $RTR$ metric is:
% % \begin{equation}
% $RTR = \sum_{i=1}^n rtr_{i}$.
% % \end{equation}
% Note that as lower the value of $RTR$ is for a given program, the better the CFI policy 
% is. The optimal value of this metric is equal to the total number of indirect return sites present 
% in the hardened program. This means that there is a one-to-one mapping.
% Other key properties:
% % \begin{itemize}
% Minimum: $RTR_{MIN} = \min_{i}{\{rtr_i\}}$;
% Maximum: $RTR_{MAX} = \max_{i}{\{rtr_i\}}$; and
% Standard Deviation (SD): $RTR_{SD} = \sqrt{\frac{\sum_{i=1}^n {(rtr_{i} - \overline{rtr_{i}})}^2}{n}}$.

% %%put afterwards in appendix
% % \begin{definition}[\textbf{CSD}]
% %  Let $ncn_{i}$ be the runtime cost for a CFI check located before an indirect callsite $ics_{i}$ which
% %  is present in a given hardened program. 
% %   Let $k$ be the runtime overhead (damping ratio) imposed by one inserted CFI check at the $irs_{i}$.
% %   The $k$ value could represent milliseconds needed to perform a CFI check.
% % \label{csd definition.}
% % \end{definition}
% % Then the $CSD$ metric is:
% % % \begin{equation}
% % $CSD = \sum_{i=1}^n ncn_{i} * k$.
% % % \end{equation}
% % Note that as lower the value of $CSD$ is for a given program, the better the CFI policy 
% % is. The optimal value of this metric is equal to the total number of indirect callsites present 
% % in the hardened program when $k$ equals one. The value of $k$ can take any millisecond value.

% %
% %%put afterwards in appendix
% % \begin{definition}[\textbf{RSD}]
% %  Let $nrn_{i}$ be the runtime cost for a CFI check performed before an indirect return site $irs_{i}$ which
% %  is present in a given hardened program. 
% %    Let $k$ be the runtime overhead (damping ratio) imposed by one inserted CFI check at the $irs_{i}$.
% %   The $k$ value could represent milliseconds needed to perform a CFI check.
% % \label{rsd definition.}
% % \end{definition}
% % Then the $RSD$ metric is:
% % % \begin{equation} 
% % $RSD = \sum_{i=1}^n nrn_{i} * k$.
% % % \end{equation}
% % Note that the lower the value of $RSD$ is for a given program, the better the CFI policy 
% % is. The optimal value of this metric is equal to the total number of indirect callsites present 
% % in the hardened program when $k$ equals one. The value of $k$ can take any millisecond value.

% \begin{definition}[\textbf{fCGA}]
% Let $cgf_{i}$ be the total number of legitimate
% call targets that are allowed and which contain gadgets according to a gadget finding tool. 
% \label{fcga definition.}
% \end{definition}
% Then the forward code reuse gadget availability $fCGA$ metric is:
% % \begin{equation}
% $fCGA = \sum_{i=1}^n cgf_{i}$.
% % \end{equation}
% Note that the lower the value of $fCGA$ is, the better the policy is. This means that
% every time a calltarget containing a code reuse gadget is protected by a CFI check, this gadget is not reachable. 
% The reverse is true when the calltarget return contains a gadget and there
% are indirect control flow transfers which can call this indirect return site unconstrained.

% %

% \begin{definition}[\textbf{bCGA}]
% Let $cgr_{i}$ be the total number of legitimate
% callee returns addresses which contain code gadgets according to a gadget finding tool. 
% \label{bcga definition.}
% \end{definition}
% Then the backward code reuse gadget availability $bCGA$ metric is:
% % \begin{equation}
% $bCGA = \sum_{i=1}^n cgr_{i}$.
% % \end{equation}
% Note that the lower the value of $bCGA$ is, the better the policy is. This means that
% every time when a calltarget return site which contains a code reuse gadget is protected by a CFI check then 
% this gadget is not reachable. The reverse is true, when the calltarget return contains a gadget and there
% are indirect control flow transfers which can call this indirect return site unconstrained.

% Above, we depicted these metrics to point out that all these CFI-related measurements
% are relevant and could be performed depending on the type of CFI policy a certain tool implements.
% The eight assessed CFI policies can neither constrain the backward edge nor analyze their availability
% of gadgets and their runtime cost.

% The metrics presented above, can be used by \sysname to assess CFI policies w.r.t. other dimensions (\textit{i.e.,} (1) backward edges, and (2) gadget availability)
% with which most of the CFI techniques are not addressing.
% Thus, we did not use the four metrics in conjunction with the eight CFI classes
% assessed in this paper since these metrics to not address (1) and (2).
% Moreover, we are not aware of any CFI policy which is based on these
% types of four metrics. Finally, by using these metrics experiments
% become more reproducible and the tools better comparable against each other.

% \section{Related Work}
% %%this section was removed from the paper in order to reach the 10 pgs max page count for the ACSAC conference.

% \textbf{\textit{Existing Metrics vs. Our Metrics.}}
% AIR~\cite{mingwei:sekar}, fAIR~\cite{vtv:tice}, and AIA~\cite{aia}
% are the only available metrics which can be used to assess the protection level offered by a CFI-based policy w.r.t. only forward-edge transfers. 
% These metrics provide average values which shed limited insight into the real 
% offered protection level. Further, these metrics can not be used to compare tools against each other since they provide average values.

% In contrast in this paper, we provide new metrics (see Appendix) for assessing not only the absolute forward-edge reduction set,
% but also the backward-edge target set reduction, the runtime damping of each CFI policy as well as the gadget availability set after a program was 
% hardened with a CFI policy.

% Additionally, two other relevant metrics are proposed by Burow \textit{et al.} \cite{cfi:survey} as follows:
% (1) qualitative metric, based on the underlying analysis provide by each of the assessed techniques, and 
% (2) quantitative metric, the product of the number of equivalence classes (EC) and the inverse of the size of the largest class (LC).

% Finally, we note that the existing forward-edge CFI metrics are mostly used without specifying the total number of callsites contained in the 
% hardened program and relating this to the total number of callsites which are protected.

% \section{Discussion}
% \textbf{Lessons Learned.}
% \label{Lessons Learned}
% First, using the same object oriented programs (OOP) concepts on which the assessed CFI-based defenses rely to build a framework 
% which gives the possibility to thoroughly reason about the assessed defenses.  
% The key observation here is that these concepts can be compartmentalized in a kind of inclusion ordering 
% w.r.t. to the size of the resulting callsite/calltarget set.
% This helps to reason more precisely about calltargets and callsites sets.

% Second, by reusing some OOP primitives offered by the compiler it offers the possibility to practically 
% reason in a consistent manner about key aspects characterizing a modeled CFI-based defense.

% % Third, looking in detail at the kind of runtime check policies which the CFI-based protection tools claim to enforce on the protected programs is another lesson we learned.
% % This helps to better classify the protection spectrum offered by each of these tools.

% Third, by carefully analyzing and comparing the residual attack surface after a defense was applied we were able to empirically confirm some common knowledge about the protection 
% level offered by certain CFI based defenses.

% Fourth, constructing a CFI-based defense assessing tool which integrates seamlessly with OOP concepts and by keeping the burden of required background
% knowledge low for the analyst is in our opinion important. 

% Finally, even the best formalization of a certain CFI defense will be not used 
% in practice if it is not simply stated and specifically tailored for the research community which mainly addresses CFI-based attack and defense topics (\textit{i.e.,} systems security, etc.). 

% % \textbf{\sysname Extensibility.}
% % \label{Extending ICFI}
